# Supplementary material for: A Tree Clock Data Structure for Causal Orderings in Concurrent Executions
Source: arXiv:2201.06325 source file (2022-01-17)
Supplement: Supplementary file 1 [file artifact_appendix.tex]

% LaTeX template for Artifact Evaluation V20201122
%
% Prepared by 
% * Grigori Fursin (cTuning foundation, France) 2014-2020
% * Bruce Childers (University of Pittsburgh, USA) 2014
%
% See examples of this Artifact Appendix in
%  * SC'17 paper: https://dl.acm.org/citation.cfm?id=3126948
%  * CGO'17 paper: https://www.cl.cam.ac.uk/~sa614/papers/Software-Prefetching-CGO2017.pdf
%  * ACM ReQuEST-ASPLOS'18 paper: https://dl.acm.org/citation.cfm?doid=3229762.3229763
%
% (C)opyright 2014-2020
%
% CC BY 4.0 license
%

%\documentclass{sigplanconf}

%\usepackage{hyperref}
%\usepackage{color}

%\begin{document}

%\special{papersize=8.5in,11in}

%%%%%%%%%%%%%%%%%%%%%%%%%%%%%%%%%%%%%%%%%%%%%%%%%%%%
% When adding this appendix to your paper, 
% please remove above part
%%%%%%%%%%%%%%%%%%%%%%%%%%%%%%%%%%%%%%%%%%%%%%%%%%%%

\appendix
\section{Artifact Appendix}

%%%%%%%%%%%%%%%%%%%%%%%%%%%%%%%%%%%%%%%%%%%%%%%%%%%%%%%%%%%%%%%%%%%%%
\subsection{Abstract}

This artifact contains all the source codes and experimental data for replicating our evaluation in Section~$6$. We implemented the analyses programs as part of the tool \textsc{Rapid}~\cite{rapid}. The provided experimental data contains all the $154$ trace logs used in our evaluation. In our artifact we also provide Python scripts that fully automate the process of replicating our evaluation.

\subsection{Artifact check-list (meta-information)} \label{sec:check-list}

%{\em Obligatory. Use just a few informal keywords in all fields applicable to your artifacts
%and remove the rest. This information is needed to find appropriate reviewers and gradually 
%unify artifact meta information in Digital Libraries.}

{\small
\begin{itemize}
  \item {\bf Algorithm: } Tree Clock
  %\item {\bf Program: } 
  %\item {\bf Compilation: }
  %\item {\bf Transformations: }
  %\item {\bf Binary: }
  %\item {\bf Model: }
  \item {\bf Data set: } Trace logs obtained from the benchmarks described in Section~$6$.
  %\item {\bf Run-time environment: }
  %\item {\bf Hardware: }
  %\item {\bf Run-time state: }
  %\item {\bf Execution: }
  \item {\bf Metrics: } Execution time.
  \item {\bf Output: } CSV files and graphs (optional).
  %\item {\bf Experiments: }
  \item {\bf How much disk space required (approximately)?: } 150 GB. 
  \item {\bf How much time is needed to prepare workflow (approximately)?:} We provide all the scripts that automate our workflow.
  \item {\bf How much time is needed to complete experiments (approximately)?: } Replicating all the results: 15 days (without parallelization). Replicating a small set of results: 1 day (without parallelization). We also provide instructions for parallelizing the computation (see Section~\ref{sec:replicating-evaluation}).
  \item {\bf Publicly available?: } Yes~\cite{zenodo}.
  \item {\bf Code licenses (if publicly available)?: } MIT License.
  \item {\bf Data licenses (if publicly available)?: } None.
  %\item {\bf Workflow framework used?: }
  \item {\bf Archived (provide DOI)?: } \href{https://doi.org/10.5281/zenodo.5749092}{doi.org/10.5281/zenodo.5749092}
\end{itemize}
}

%%%%%%%%%%%%%%%%%%%%%%%%%%%%%%%%%%%%%%%%%%%%%%%%%%%%%%%%%%%%%%%%%%%%%
\subsection{Description}

\subsubsection{How to access}\label{sec:how-to-access}

Obtain the artifact from~\cite{zenodo}. The total size is expected to be approximately 50 MB. 

\subsubsection{Hardware dependencies}
Replicating the results of large benc\-hmarks requires up to 30 GB RAM. Otherwise, there are no special hardware requirements for using our artifact.

\subsubsection{Software dependencies}\label{sec::software-dep}
Java 11, Ant 1.10 or higher, Python 3.7 or higher, including the packages pandas and matplotlib. 

\subsubsection{Data sets}\label{sec:data-set}
The trace logs are available for download at~\cite{tracelogs}.

%\subsubsection{Models}

%%%%%%%%%%%%%%%%%%%%%%%%%%%%%%%%%%%%%%%%%%%%%%%%%%%%%%%%%%%%%%%%%%%%%
\subsection{Installation}

Obtain the artifact (see Section~\ref{sec:how-to-access}), extract the archive files and set the \texttt{\$AE\_HOME} environment variable:

\texttt{> export AE\_HOME=/path/to/AE}

Next, install \textsc{Rapid}:

\texttt{> cd \$AE\_HOME/rapid/}\\
\texttt{> ant jar}

Then, download the benchmark traces (see Section~\ref{sec:data-set}) into the folder \texttt{\$AE\_HOME/benchmarks/}. 

%%%%%%%%%%%%%%%%%%%%%%%%%%%%%%%%%%%%%%%%%%%%%%%%%%%%%%%%%%%%%%%%%%%%%
\subsection{Experiment workflow}

In Figure~\ref{fig:dir-structure} we display the directory structure of our artifact. The directory \texttt{rapid} contains the \textsc{Rapid} tool which includes our implementation of the tree clock and vector clock data structures and the analyses programs based on HB, SHB and MAZ partial orders. The directory \texttt{benchmarks} is designated for the trace logs. The directory \texttt{scripts} contains a collection of helper scripts that automate our workflow. In particular, the script \texttt{\$AE\_HOME/scripts/run.py} can be utilized to automate the process of replicating the results of Section~\ref{sec:experiments}. In Section~\ref{sec:replicating-evaluation} we describe how the script can be used to replicate all or part of our experimental evaluation. In addition, Section~\ref{sec:experiment-custom} contains instructions on how the script can be used to evaluate a new trace log that is not part of the original benchmark set. The \texttt{README.md} file provides more comprehensive information on certain aspects of our artifact.

\begin{figure}
    \centering
\begin{verbatim}
AE_HOME/
|--- rapid/
|--- benchmarks/
|--- scripts/
|--- results/
|--- LICENSE.txt
|--- README.md
\end{verbatim}
    \caption{Directory structure of the artifact}
    \label{fig:dir-structure}
\end{figure}

%%%%%%%%%%%%%%%%%%%%%%%%%%%%%%%%%%%%%%%%%%%%%%%%%%%%%%%%%%%%%%%%%%%%%
\subsection{Evaluation and expected results}\label{sec:replicating-evaluation}

%\subsubsection{Getting Started}
%Running the script with \texttt{python \$AE\_HOME/scripts/run.py -{}-test} will run the analyses on the trace logs under \texttt{\$AE\_HOME/benchmarks/test/} and generate CSV files as output under \texttt{\$AE\_HOME/results/test/}. The expected results of this evaluation is outlined in the file \texttt{\$AE\_HOME/benchmarks/test/expected\_results.txt}. Note that these trace logs are included for performing a sanity check on the installation and are not part of the experimental evaluation of Section~\ref{sec:experiments}. 

%\subsubsection{Replicating the Evaluation}
Executing the following command will run all the analyses on all the trace logs:

\texttt{> python \$AE\_HOME/scripts/run.py -b all} 

The outputs of the executions will be extracted as CSV files under the folder \texttt{\$AE\_HOME/results/}. Note that this command expects to locate all the benchmarks used in our evaluation (see Section~\ref{sec:data-set}) under the folder \texttt{\$AE\_HOME/benchmarks/}. 

The main goal of this evaluation is to measure the performance benefits of tree clocks over vector clocks for keeping track of logical times in concurrent programs. We expect that the overall speedup would remain similar to the speedups reported in Table~\ref{tab:speedups} for each category. After the CSV output files have been generated, the script \texttt{\$AE\_HOME/scripts/compute\_averages.py} may be utilized to compute the average speedup for each category and replicate the Table~\ref{tab:speedups}:

\texttt{> python \$AE\_HOME/scripts/compute\_averages.py\\ \$AE\_HOME/results/} 

This script expects the path to the results folder as argument and outputs a file named \texttt{table2.csv} under the same folder that replicates the Table~\ref{tab:speedups}. Similarly, the script \texttt{\$AE\_HOME/scripts/plot.py} can be utilized to visualize the obtained outputs and replicate the Figure~\ref{fig:time_comparison}:

\texttt{> python \$AE\_HOME/scripts/plot.py \$AE\_HOME/results/} 

This script also expects the path to the results folder as argument and outputs the plot files under the folder \texttt{\$AE\_HOME/results/\allowbreak plots} that replicates Figure~\ref{fig:time_comparison}. 

We remark that, as also indicated in Section~\ref{sec:check-list}, replicating the evaluation can take very long if executed serially. We refer the interested readers to the file \texttt{\$AE\_HOME/README.md} where we describe a procedure which may be utilized to parallelize the evaluation. Furthermore, the script \texttt{\$AE\_HOME/scripts/run.py} also provides an option to replicate only parts of our experimental evaluation. The following command runs the analyses on a small set of benchmarks which require moderate system resources and reduced computation time (see Section~\ref{sec:check-list}):

\texttt{> python \$AE\_HOME/scripts/run.py -b small}

We refer the readers to the \texttt{\$AE\_HOME/README.md} file for more detailed information on customizing the experiments. 
%%%%%%%%%%%%%%%%%%%%%%%%%%%%%%%%%%%%%%%%%%%%%%%%%%%%%%%%%%%%%%%%%%%%%
\subsection{Experiment customization}\label{sec:experiment-custom}
Users might utilize the script \texttt{\$AE\_HOME/scripts/run.py} to evaluate a new trace log that is not part of our original benchmark set. This can be achieved with the following command:

{\texttt{> python \$AE\_HOME/scripts/run.py -p path/to/trace -n output-folder-name}
}

The above command will run all the analyses on the input trace located in \texttt{path/to/trace} and extract the output CSV files into \texttt{\$AE\_HOME/results/output-folder-name}. Note that the given input trace must be in one of the formats admitted by the \textsc{Rapid} tool. Readers may refer to the \texttt{\$AE\_HOME/rapid/README.md} file for information regarding the formats admitted by \textsc{Rapid}. 
%%%%%%%%%%%%%%%%%%%%%%%%%%%%%%%%%%%%%%%%%%%%%%%%%%%%%%%%%%%%%%%%%%%%%
\subsection{Notes}
We note that the reported execution times correspond to the time taken for performing the respective analyses and do not include the time taken for processing the input files. Hence, the actual execution times are expected to be longer than the reported times.   

%HB Race: FastHBVectorClock, FastHBTreeClockAL
%HB No Race: HBNoRace, HBTreeClockNoRaceAL 

%SHB Race: SHBEpoch, SHBEpochTreeClockAL
%SHB No Race: SHBNoRace, SHBTreeClockNoRaceAL

%MAZ Race: MAZVectorClockRaceDetection, MAZTreeClockRaceDetection 
%MAZ No Race: MAZVectorClockNoRace, MAZTreeClockNoRace 

%%%%%%%%%%%%%%%%%%%%%%%%%%%%%%%%%%%%%%%%%%%%%%%%%%%%%%%%%%%%%%%%%%%%%
\iffalse
\subsection{Methodology}

Submission, reviewing and badging methodology:

\begin{itemize}
  \item \url{https://www.acm.org/publications/policies/artifact-review-badging}
  \item \url{http://cTuning.org/ae/submission-20201122.html}
  \item \url{http://cTuning.org/ae/reviewing-20201122.html}
\end{itemize}

%%%%%%%%%%%%%%%%%%%%%%%%%%%%%%%%%%%%%%%%%%%%%%%%%%%%
% When adding this appendix to your paper, 
% please remove below part
%%%%%%%%%%%%%%%%%%%%%%%%%%%%%%%%%%%%%%%%%%%%%%%%%%%%
\fi

%\end{document}
