# Supplementary material for: A Tree Clock Data Structure for Causal Orderings in Concurrent Executions
Source: arXiv:2201.06325 source file (2022-01-17)
Supplement: Supplementary file 2 [file appendix.tex]

\input{proofs}
\input{hb_example}
